# Supplementary material for: Evaluation for Weakly Supervised Object Localization: Protocol, Metrics, and Datasets
Source: arXiv:2007.04178 source file (2021-12-07)
Supplement: Supplementary file 1 [file appendix.tex]

\addcontentsline{toc}{section}{Appendices}
%\part*{Appendix}
\appendix

We include additional materials in this document. Each section matches with the main paper sections: \S\ref{appendix:problem_formulation} to main paper \S\ref{sec:wsol_impossibility}, \S\ref{appendix:evaluation_protocol} to main paper \S\ref{sec:evaluation}, and \S\ref{appendix:experiments} to main paper \S\ref{sec:results}.

\section{Problem Formulation of WSOL}
\label{appendix:problem_formulation}

\subsection{CAM as patch-wise posterior approximation}
\label{appendix:cam_as_posterior_approximation}

In the main paper \S\ref{subsec:what_is_wsol}, we have described class activation mapping (CAM)~\cite{CAM} as a patch-wise posterior approximator trained with image-level labels. We describe in detail why this is so. 

\myparagraph{Equivalent re-formulation of CAM.}
Originally, CAM is a technique applied on a convolutional neural network classifier $h:\mathbb{R}^{3\times H \times W}\rightarrow\mathbb{R}^{C}$, where $C$ is the number of classes, of the following form:
\begin{equation}
    h_{c}(X)=\sum_{d}W_{cd}\left(\frac{1}{HW}\sum_{ij}g_{dij}(\mathbf{X})\right)
\end{equation}
where $c,d$ are the channel-dimension indices and $i,j$ are spatial-dimension indices. In other words, $h$ is a fully convolutional neural network, followed by a global average pooling (GAP) and a linear (fully-connected) layer into a $C$-dimensional vector. We may swap the GAP and linear layers without changing the representation:
\begin{align}
    h_{c}(X)
    &=\frac{1}{HW}\sum_{ij}\left(\sum_{d}W_{cd}g_{dij}(\mathbf{X})\right) \\
    &=:\frac{1}{HW}\sum_{ij}f_{cij}(\mathbf{X}) 
\end{align}
where $f$ is now a fully-convolutional network. Each pixel $(i,j)$ in the feature map, $\left(f_{1ij}(\mathbf{X}),\cdots,f_{Cij}(\mathbf{X})\right)$, corresponds to the classification result of the corresponding field of view in the input $\mathbf{X}$, written as $X_{ij}$. Thus, we equivalently write \begin{align}
    h_{c}(X)=\frac{1}{HW}\sum_{ij}f_{c}(X_{ij}) 
\end{align}
where $f$ is now re-defined as a image patch classifier with 1-dimensional feature output (not fully convolutional).

\myparagraph{CAM as patch-wise posterior approximator.}
$h$ is now the average-pooled value of the patch-wise classification scores $f_{c}(X_{ij})$. CAM trains $f$ by maximizing the image-wide posterior of the ground truth class, where the posterior is defined as the softmax over $f(X_{ij})$:
\begin{equation}
    \log p(Y|\mathbf{X}):=
    \log \text{softmax}^Y\left(\frac{1}{HW}\sum_{ij}f(X_{ij})\right).
\end{equation}
In other words, CAM trains the network for patch-wise scores $f_{c}(X_{ij})$ to estimate the image-wide posterior $p(Y|\mathbf{X})$. 

At inference time, CAM estimates the pixel-wise posterior $p(Y|X_{ij})$ approximately by performing $p(Y|X_{ij})\approx f_Y(X_{ij})/\max_{\alpha\beta}f_Y(X_{\alpha\beta})$ (modulo some calibration to make sure $p(Y|X_{ij})\in [0,1]$).

\subsection{Proof for the ill-posedness lemma}
\label{appendix:proof}

We first define an evaluation metric for our score map for an easier argumentation. 
\begin{definition}
For a scoring rule $s$ and a threshold $\tau$, we define the \textbf{pixel-wise localization accuracy} $\text{\pxacc}(s,\tau)$ as the probability of correctly predicting the pixel-wise labels:
\begin{align}
    \text{\pxacc}(s,\tau)=
    {P}_{X,T}(s(X)\geq\tau\mid T=1)\cdot{P}_{X,T}(T=1)
    \nonumber\\
    +{P}_{X,T}(s(X)<\tau\mid T=0)\cdot{P}_{X,T}(T=0)
    \nonumber
\end{align}
\end{definition}
We prove the following lemma.
\begin{lemma}
    Assume that the true posterior $p(Y|M)$ with a continuous pdf is used as the scoring rule $s(M)=p(Y|M)$. Then, there exists a scalar $\tau\in\mathbb{R}$ such that $\text{\pxacc}(p(Y|M),\tau)=1$ if and only if the foreground-background posterior ratio $\frac{p(Y=1|M^{\text{fg}})}{p(Y=1| M^{\text{bf}})}\geq 1$ almost surely, conditionally on the event $\{T(M^{\text{fg}})=1\text{ and }T(M^{\text{bf}})=0\}$.
\end{lemma}
\begin{proof}

    We write $E:=\{T(M^{\text{fg}})=1\text{ and }T(M^{\text{bf}})=0\}$.
    
    \noindent
    (\textbf{Proof for ``if''}) Assume $\alpha\geq 1$ almost surely, given $E$. Let
    \begin{align}
        \tau:=\min_{G:P(G\Delta \{T(m)=0\})=0}\,\,
        \max_{m\in G}\,\,
        p(Y=1| M=m)
    \end{align} 
    where $\Delta$ is the set XOR operation: $A\Delta B:=(A\cup B)\setminus (A\cap B)$. Then, for almost all $M^{\text{fg}},M^{\text{bg}}$ following $E$, 
    \begin{align}
        p(Y=1| M^{\text{fg}})\geq \tau \geq p(Y=1| M^{\text{bg}}).
        \label{eq:co_occurrence_ordered}
    \end{align}
    Therefore, 
    \begin{align}
        &P(p(Y=1| M^{\text{fg}})\geq \tau\mid T(M^{\text{fg}})=1)\nonumber\\
        &=P(p(Y=1| M^{\text{bg}})\leq \tau\mid T(M^{\text{bg}})=0) =1
        \label{eq:loc_conditionals_prob_1}
    \end{align}
    and so $\text{\pxacc}(p(Y|M),\tau)=1$.
    
    \noindent
    (\textbf{Proof for ``only if''}) Assume $\text{\pxacc}(p(Y| M),\tau)=1$ for some $\tau$. W.L.O.G., we assume that ${P}(T(M)=1)\neq 0$ and ${P}(T(M)=0)\neq 0$ (otherwise, ${P}(E)=0$ and the statement is vacuously true). Then, Equation~\ref{eq:loc_conditionals_prob_1} must hold to ensure $\text{\pxacc}(p(Y| M),\tau)=1$. Equation~\ref{eq:co_occurrence_ordered} then also holds almost surely, implying $\alpha\geq 1$ almost surely.
\end{proof}

\subsection{Foreground-background posterior ratio}
\label{appendix:fg_bg_posterior_ratio}

We have described the the pathological scenario for WSOL as when the foreground-background posterior ratio $\alpha$ is small (\S3.2). We discuss in greater detail what it means and whether there are data-centric approaches to resolve the issue. For quick understanding, assume the task is the localization of duck pixels in images. The foreground cue of interest $M^{\text{fg}}$ is ``feet'' of a duck and background cue of interest $M^{\text{bg}}$ is ``water''. Then, we can write the posterior ratio as
{
\begin{equation}
    \alpha:=
    \frac{p(\eqd|\eqf)}{p(\eqd|\eql)}= 
    \frac{p(\eqf|\eqd)}{p(\eql|\eqd)} \cdot \left(\frac{p(\eqf)}{p(\eql)}\right)^{-1}
    \nonumber
\end{equation}
$\alpha<1$ implies that lake patches are more abundant in duck images than are duck's feet (see Figure~\ref{fig:duck_feet_lake_appendix}) for an illustration. 

\begin{figure}
    \centering
    \includegraphics[width=\linewidth]{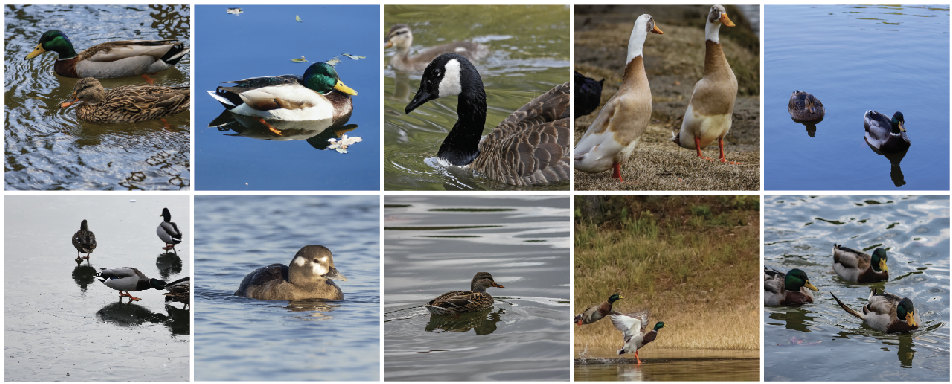}
    \caption{\small\textbf{Ducks.} Random duck images on Flickr. They contain more lake than feet pixels: $p(\eql|\eqd)\gg p(\eqf|\eqd)$.}
    \label{fig:duck_feet_lake_appendix}
\end{figure}

To increase $\alpha$, two approaches can be taken. (1) Increase the likelihood ratio $\frac{p(\eqf|\eqd)}{p(\eql|\eqd)}$. This can be done by collecting more images where duck's feet have more pixels than lake does. (2) Decrease the prior ratio $\frac{p(\eqf)}{p(\eql)}$. Note that the prior ratio can be written
\begin{equation}
\footnotesize
    \frac{p(\eqf)}{p(\eql)}=
    \frac{p(\eqf|\eqd)p(\eqd)+p(\eqf|\eqnd)p(\eqnd)}%
    {p(\eql|\eqd)p(\eqd)+p(\eql|\eqnd)p(\eqnd)}
    \nonumber
\end{equation}
With fixed likelihoods $p(\eqf|\eqd)$ and $p(\eql|\eqd)$, one can decrease the prior ratio by increasing the likelihood of lake cues in non-duck images $p(\eql|\eqnd)$. We can alter WSOL into a more well-posed task also by including many background images containing confusing background cues.

Such data-centric approaches are promising future research directions for turning WSOL into a well-posed task. 
}

\section{Evaluation Protocol for WSOL}
\label{appendix:evaluation_protocol}

\subsection{Score map normalization}
\label{appendix:score_map_normalization}

A common practice in WSOL is to normalize the score maps per image because the maximal (and minimal) scores differ vastly across images. Prior WSOL papers have introduced either max normalization (dividing through by $\max_{ij}s_{ij}$) or min-max normalization (additionally mapping $\min_{ij}s_{ij}$ to zero). After normalization, WSOL methods threshold the score map at $\tau$ to generate a tight box around the binary mask $\{(i,j)\mid s_{ij}\geq \tau\}$. $\tau$ is typically treated as a fixed value~\cite{CAM,ACoL,CutMix} or a hyperparameter to be tuned~\cite{HaS,SPG,ADL}. We summarize that how prior works calibrate and threshold score maps in Table \ref{tab:prior_wsol_operating_thresholds}. As discussed in \S\ref{subsec:evaluation_metrics} of main paper, we use the min-max normalization.

\begin{table}
    \newcommand\maxnormf{\overline{s}_{ij}}
    \newcommand\minmaxnormf{\widehat{s}_{ij}}
    \small
    \centering
    \begin{tabular}{*{2}{l}*{2}{l}}
         Method && Paper & Code  \\
         \cline{1-1} \cline{3-4}
         \vspace{-1em} & \\
         \cline{1-1} \cline{3-4}
         \vspace{-1em} & \\
         CAM~\cite{CAM} && $\maxnormf\geq 0.2$ & $\maxnormf\geq 0.2$ \\
         HaS~\cite{HaS} && Follow CAM$^\dagger$ & Follow CAM \\
         ACoL~\cite{ACoL} && Follow CAM & $\minmaxnormf\geq \text{unknown}$ \\
         SPG~\cite{SPG} && Grid search threshold & $\minmaxnormf\geq \text{unknown}$ \\
         ADL~\cite{ADL} && Not discussed & $\minmaxnormf\geq 0.2^\dagger$ \\
         CutMix~\cite{CutMix} && $\maxnormf\geq 0.15$ & $\minmaxnormf\geq 0.15$ \\
         \cline{1-1} \cline{3-4}
         \vspace{-1em} & \\
         Our protocol && $\minmaxnormf\geq \tau^\star$ & $\minmaxnormf\geq \tau^\star$ \\
         \cline{1-1} \cline{3-4}
    \end{tabular}
\[
\overline{s}_{ij}:=\frac{s_{ij}}{\max_{kl}s_{kl}}\quad \quad \widehat{s}_{ij}:=\frac{s_{ij}-\min_{kl}s_{kl}}{\max_{kl}s_{kl}-\min_{kl}s_{kl}}
\]
    \caption{\small \textbf{Calibration and thresholding in WSOL.} Score calibration is done per image: max ($\overline{s}_{ij}$) or min-max ($\widehat{s}_{ij}$) normalization. Thresholding is required only for the box evaluation. $\tau^\star$ is the optimal threshold (\S\ref{subsec:evaluation_metrics} in main paper). Daggers ($^\dagger$) imply that the threshold depends on the backbone architecture.}
    \label{tab:prior_wsol_operating_thresholds}
\end{table}

\subsection{Data preparation}
\label{appendix:data}

We present the following data-wise contributions in this paper (contributions \textbf{bolded}):
\begin{itemize}
    \item CUB: \textbf{New data} (5 images per class) with \textbf{bounding box annotations}.
    \item ImageNet: ImageNetV2~\cite{ImageNetV2} with new \textbf{bounding box annotations}.
    \item OpenImages: \textbf{Processed} a split for the WSOL training, hyperparameter search, and evaluation with ground truth object masks.
\end{itemize}

\subsubsection{ImageNet}
\label{appendixsub:imagenet}

The \textit{test set} of ImageNet-1k dataset~\cite{ImageNet} is not available. Therefore, many researchers report the accuracies on the \textit{validation set} for their final results~\cite{CutMix}. Since this practice may let models overfit to the evaluation split over time, ImageNetV2~\cite{ImageNetV2} has been proposed as the new test sets for ImageNet-1k trained models. ImageNetV2 includes three subsets according to the sampling strategies, \texttt{MatchedFrequency}, \texttt{Threshold0.7}, and \texttt{TopImages}, each with $10\,000$ images ($10$ images per class). We use the \texttt{Threshold0.7} split as our \trainfullsup. Since ImageNetV2 does not contain localization supervision, we have annotated bounding boxes on those images, following the annotation protocol of ImageNet. The total number of annotated bounding boxes are $18\,532$.

\subsubsection{CUB}
\label{appendixsub:cub}

We have collected 5 images for each of the 200 CUB fine-grained bird classes from Flickr. The overall procedure is summarized as:

\begin{enumerate}
    \item Crawl images from Flickr.
    \item De-duplicate images.
    \item Manually prune irrelevant images (three people).
    \item Prune with model classification scores.
    \item Resize images.
    \item Annotate bounding boxes.
\end{enumerate}

\myparagraph{Crawl images from Flickr.}
Since original CUB itself is collected from Flickr, we use Flickr as the source of bird images. We have used the \texttt{Flickr API}\footnote{\url{https://www.flickr.com/services/api/}} to crawl up to 400 images per class with class name as search terms. We have only crawled images under the following licenses: 
\begin{itemize}
    \item \texttt{Attribution}
    \item \texttt{Attribution-NonCommercial}
    \item \texttt{Public Domain Dedication}
    \item \texttt{Public Domain Mark}
\end{itemize}

\myparagraph{De-duplicate images.}
We de-duplicate the images using the \texttt{ImageHash} library\footnote{\url{https://pypi.org/project/ImageHash/}} first among the crawled images themselves and then against the training and test splits of CUB.

\myparagraph{Manually prune irrelevant images (three people).}
Since crawled images of each class contain negative-class images (non birds and birds of wrong categories), three humans have participated in the prune-out process. We have only kept the images that all three have voted for ``positive''.

\myparagraph{Prune with model classification scores.}
To match with the original CUB data distribution, we have trained a fine-grained bird classifier using ResNet50~\cite{ResNet} on the CUB training split. Among crawled images, those with ground truth class confidence scores lower than 0.5 have been pruned out.

\myparagraph{Achieving 5 images per class.}
At this point, most classes have more than 5 images per class and a few have less than 5. In the former case, we have randomly sampled 5 images per class. 

\myparagraph{Resize images.}
Photographic technologies have made significant advances over the decade since the time original CUB was collected. As a result, image size statistics differ. To fix this, we have resized the images appropriately.

\myparagraph{Annotate bounding boxes.}
The evaluation on CUB is based on bounding boxes. Thus, the held-out set images are supplied with tight bounding boxes around birds (one per image).

\begin{figure}
    \centering
    \includegraphics[width=\linewidth]{figures/appendix/cub_v2.png}
    \caption{\small \textbf{CUB version 2.} Sample images.}
    \label{fig:cub_v2_samples}
\end{figure}

\subsubsection{OpenImages}
\label{appendixsub:openimages}
There are three significant differences between OpenImagesV5~\cite{OpenImagesV5} and CUB or ImageNet that make the OpenImages not suitable as a WSOL benchmark in its original form. (1) Images are multi-labeled; it is not sensible to train classifiers with the standard softmax cross-entropy loss assuming single label per image. (2) OpenImages has less balanced label distributions. (3) There are nice instance segmentation masks, but they have many missing instances.

We have therefore processed a subset of OpenImages into a WSOL-friendly dataset where the above three issues are resolved. The procedure is as follows:
\begin{enumerate}
    \item Prune multi-labeled samples.
    \item Exclude classes with not enough samples.
    \item Randomly sample images for each class.
    \item Prepare binary masks.
    \item Introduce ignore regions.
\end{enumerate}

\myparagraph{Prune multi-labeled samples.}
We prune the multi-labeled samples in the segmentation subset of OpenImages.
This process rejects 34.5\% samples in OpenImages.

\myparagraph{Exclude classes with not enough samples.}
After pruning multi-label samples, some classes are not available in validation and test sets. We have first defined the minimum number of samples per classes as (300, 25, 50) for (train, validation, test), and have excluded classes that do not meet the minimum requirement, resulting in 100 classes (out of 350 original classes).

\myparagraph{Randomly sample images for each class.}
We have randomly sampled (300, 25, 50) samples per class for (train, validation, test). This eventually results in $29\,819$ \trainweaksup (train), $2\,500$ \trainfullsup (validation), and $5\,000$ \testfullsup (test) samples.

\myparagraph{Prepare binary masks.}
WSOL methods are evaluated against binary masks of the foreground category in each image. Since OpenImages comes with instance-level masks of various categories, we have taken the union of instance masks of the class of interest in every image to build the binary masks.

\begin{figure}
    \centering
    \includegraphics[width=\linewidth]{figures/appendix/openimages_sample_4e993aed623ea5e2.png}
    \caption{\small \textbf{OpenImages V5 sample.} Example of ``group-of'' box annotations. There is only one ``Book'' mask in the left bottom corner.}
    \label{fig:openimage_group_of_sample}
\end{figure}

\myparagraph{Introduce ignore regions.}
OpenImages has instance-wise masks, but not all of them are annotated as masks. When the objects are difficult to be annotated instance-wise or there are simply too many, the ``group-of'' box annotations are provided over the region containing multiple instances (\eg hundreds of books on bookshelves in an image taken at a library -- See Figure~\ref{fig:openimage_group_of_sample}). We have indicated the regions with the ``group-of'' boxes as ``ignore'' regions, and have excluded them from the evaluation during the computation of \pxprec, \pxrec, and \pxap.

\subsection{Transferability of rankings between \trainfullsup and \testfullsup}
\label{appendix:trainfullsup_testfullsup_transfer}

As detailed in main paper \S\ref{subsec:evaluation_benchmarks}, we search hyperparameters on \trainfullsup and test them on \testfullsup. To validate if the found hyperparameter rankings do transfer well between the splits, we show the preservation of ranking statistics in Table~\ref{tab:supp-val-test-transfer} and visualize the actual rankings in Figure~\ref{fig:val-test-ranking_preservation}. We observe that the rankings are relatively well-preserved (with Kendall's tau values $>0.7$).

\input{tables/kendall.tex}

\subsection{Hyperparameter search with proxy \trainweaksup}
\label{appendix:okay_to_use_proxy_imagenet}

We have reduced the training set size (\trainweaksup) to 10\% for ImageNet hyperparameter search for the interest of computational efficiency (\S4.2). We examine how much this reduction affects the rankings of hyperparameters. We show a similar analysis as in \S\ref{appendix:trainfullsup_testfullsup_transfer}: see Figure~\ref{fig:proxy-imagenet}. We observe again that with Kendall's tau value $0.743$, the two rankings are largely preserved.

\begin{figure}
    \centering
    \includegraphics[width=\linewidth]{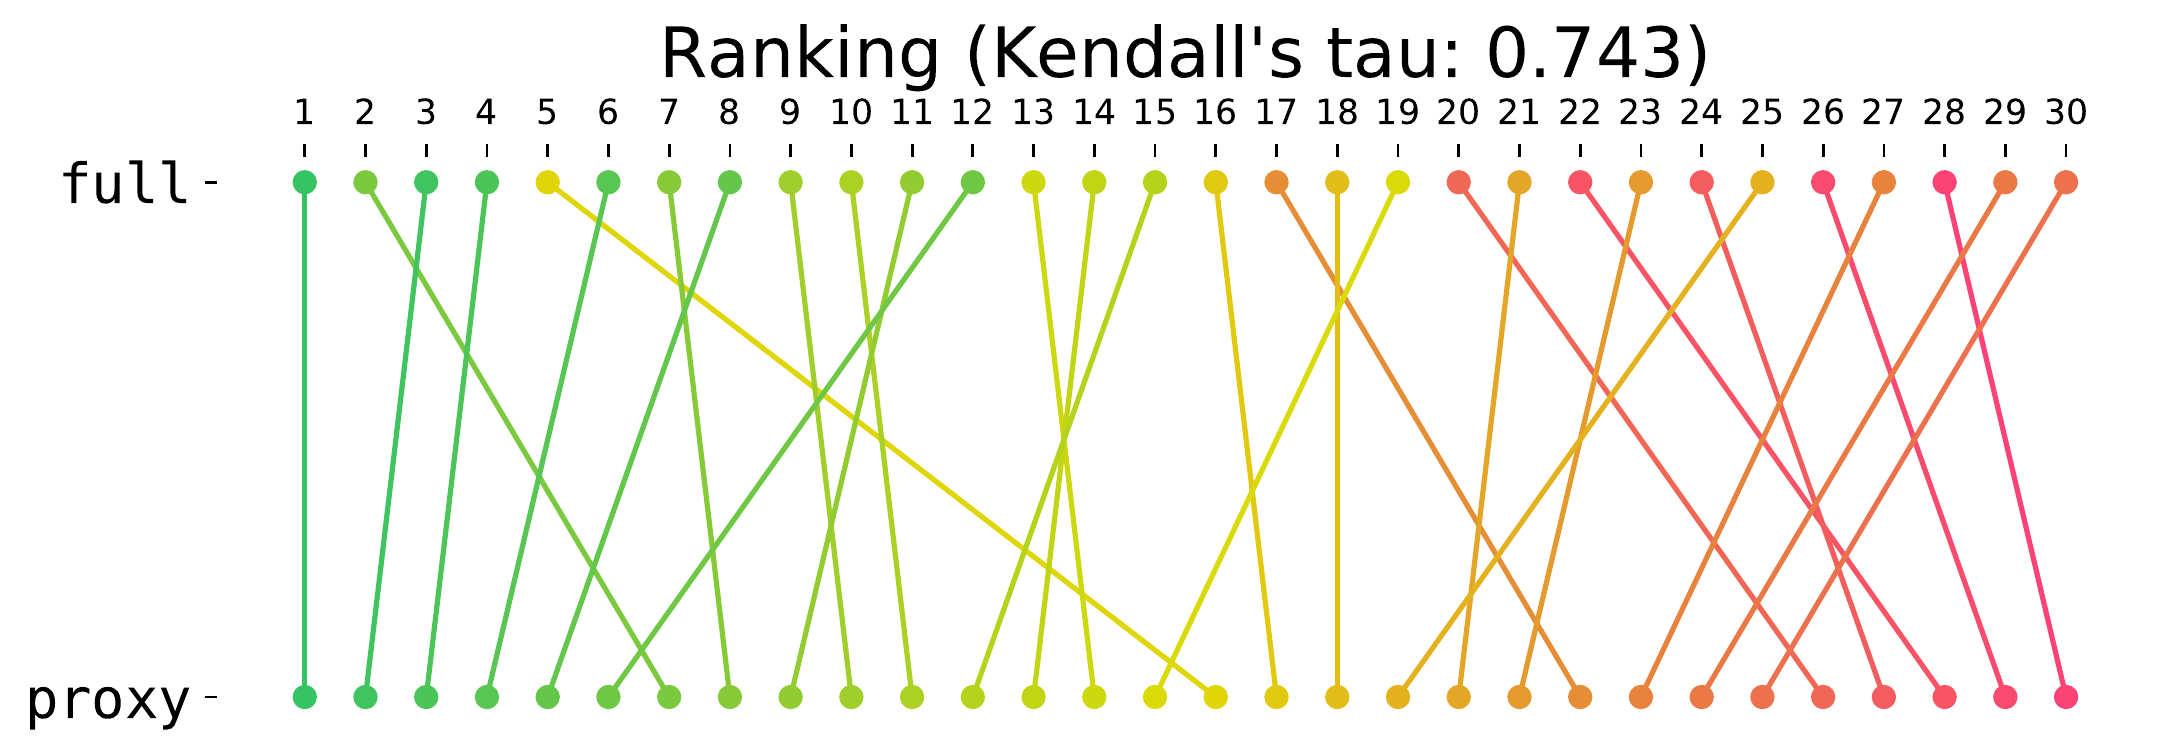}
    \caption{\small \textbf{Proxy ImageNet ranking}. Ranking of hyperparameters is largely preserved between the models trained on the full \trainweaksup and its 10\% proxy. Kendall's tau is $0.743$.}
    \label{fig:proxy-imagenet}
\end{figure}

\section{Experiments}
\label{appendix:experiments}

\subsection{Prior WSOL methods and hyperparameters}
\label{appendix:wsol_methods}

\begin{table}
    \footnotesize
    \centering
    \begin{tabular}{cccc}
        Methods && Hyperparameter & Distribution  \\
        \cline{1-1} \cline{3-4}
        \vspace{-1em} & \\
        \cline{1-1} \cline{3-4}
        \vspace{-1em} & \\
        Common && Learning rate & $\text{LogUniform}[10^{-5},10^0]$ \\
        && Score-map resolution & $\text{Categorical}\{14,28\}$ \\
        \cline{1-1} \cline{3-4}
        \vspace{-1em} & \\
        HaS~\cite{HaS} && Drop rate & $\text{Uniform}[0,1]$ \\
        && Drop area & $\text{Uniform}[0,1]$  \\
        \cline{1-1} \cline{3-4}
        \vspace{-1em} & \\  
        ACoL~\cite{ACoL} && Erasing threshold & $\text{Uniform}[0,1]$ \\
        \cline{1-1} \cline{3-4}
        \vspace{-1em} & \\
        SPG~\cite{SPG} && Threshold $\delta_{l}^{B1}$ & $\text{Uniform}[0,1]$ \\
            && Threshold $\delta_{h}^{B1}$ & $\text{Uniform}[\delta_{l}^{B1},1]$ \\
            && Threshold $\delta_{l}^{B2}$ & $\text{Uniform}[0,1]$ \\
            && Threshold $\delta_{h}^{B2}$ & $\text{Uniform}[\delta_{l}^{B2},1]$ \\
            && Threshold $\delta_{l}^{C}$ & $\text{Uniform}[0,1]$ \\
            && Threshold $\delta_{h}^{C}$ & $\text{Uniform}[\delta_{l}^{C},1]$ \\
        \cline{1-1} \cline{3-4}
        \vspace{-1em} & \\
        ADL~\cite{ADL} && Drop rate & $\text{Uniform}[0,1]$ \\
        && Erasing threshold & $\text{Uniform}[0,1]$ \\
        \cline{1-1} \cline{3-4}
        \vspace{-1em} & \\
        CutMix~\cite{CutMix} && Size prior & $\frac{1}{\text{Uniform}(0,2]}-\frac{1}{2}$ \\
        && Mix rate & $\text{Uniform}[0,1]$ \\
        \cline{1-1} \cline{3-4}
    \end{tabular}
    \vspace{1em}
    \caption{\small \textbf{Hyperparameter search spaces.} }
    \label{tab:hyperparameter_list}
\end{table}

We describe each method in greater detail here. The list of hyperparameters for each method is in Table~\ref{tab:hyperparameter_list}.

\input{tables/main_results_cls.tex}
\input{tables/all_wsol_results_vir.tex}

\paragraph{CAM, CVPR'16~\cite{CAM}.}
Class Activation Mapping trains a classifier of fully-convolutional backbone with global average pooling structure, and at test time uses the logit outputs before the global average pooling for the scoring rule $s(X_{ij})$. See Appendix~\S\ref{appendix:cam_as_posterior_approximation} for the interpretation of CAM as a posterior approximator. CAM has learning rate (LR) and the score-map resolution (SR) as hyperparameters. LR is sampled log-uniformly from $[10^{-5},10^{0}]$, where end points correspond roughly to ``no training'' and ``training always diverges'' cases. SR is sampled from $\text{Categorical}\{14,28\}$, two widely used resolutions in prior WSOL methods. All five methods below use CAM technique in the background, and have LR and HR as design choices.

\paragraph{HaS, ICCV'17~\cite{HaS}.}
Hide-and-Seek (HaS) is a data augmentation technique that divides an input image into grid-like patches, and then randomly select patches to be dropped. The hyperparameters of HaS are drop rate (DR) and drop area (DA). Specifically, the size of each patch is decided by DA, and the probability of each patch to be selected for erasing is decided by DR. DA is sampled from a uniform distribution $U[0,1]$, where $0$ corresponds to ``no grid'' and $1$ indicates ``full image as one patch''.

\paragraph{ACoL, CVPR'18~\cite{ACoL}.}
Adversarial Complementary Learning (ACoL) adds one more classification head to backbone networks. From one head, ACoL finds the high-score region using CAM using erasing threshold (ET) and erases it from an internal feature map. The other head learns remaining regions using the erased feature map. We sample ET from a uniform distribution $U[0,1]$, where $0$ means ``erasing whole feature map'' and $1$ means ``do not erase''.

\paragraph{SPG, ECCV'18~\cite{SPG}.}
Self-produced Guidance (SPG) utilizes spatial information about fore- and background using three additional branches (\texttt{SPG-B1,B2,C}). To divide foreground and background from score-map, they introduce two hyperparameters, $\delta_{l}$ and $\delta_{h}$, per each branch. When the score is lower than $\delta_{l}$, the pixel is considered as background, and the pixel is considered as foreground when the score is higher than  $\delta_{h}$. The remaining region (higher than $\delta_{l}$, lower than  $\delta_{h}$) is ignored. We first sample $\delta_{l}$ from $U[0,1]$, and then $\delta_{h}$ is sampled from $U[\delta_{l},1]$.

\paragraph{ADL, CVPR'19~\cite{ADL}.}
Attention-based Dropout Layer (ADL) is a block applied on an internal feature map during training. ADL produces a drop mask by finding the high-score region to be dropped using another scoring rule~\cite{zagoruyko2017paying}. Also, ADL produces an importance map by normalizing the score map and uses it to increase classification power of the backbone. At each iteration, only one component is applied between the drop mask and importance map. The hyperparameters of ADL are drop rate (DR) that indicates how frequently the drop mask is selected and erasing threshold (ET) that means how large regions are dropped. We sample DR and ET from uniform distributions $U[0,1]$.

\paragraph{CutMix, ICCV'19~\cite{CutMix}.}
CutMix is a data augmentation technique, where patches in training images are cut and paste to other images and target labels are mixed likewise. Its hyperparameters consist of the size prior $\alpha$ (used for sampling sizes according to $\sim\!\!\text{Beta}(\alpha,\alpha)$) and the mix rate $r$ (Bernoulli decision for ``CutMix or not''). The size prior is sampled from the positive range $\frac{1}{\text{Unif}(0,2]}-\frac{1}{2}$; then, $\text{Var}(\text{Beta}(\alpha,\alpha))$ follows the uniform distribution between 0 and 0.25 (maximal variance; two Dirac deltas at 0 and 1).

\subsection{Classification results of WSOL methods}
\label{appendix:cls_performance}

The widely-used ``top-1 localization accuracy'' for WSOL represents both the classification \textit{and} localization performances. The metric can be misleading as a localization metric, as the increase in numbers can also be attributed to the improved classification accuracies. Thus, in the main paper, we have suggested using on the ``GT-known'' type of metrics like \maxboxacc and \pxap that measures the localization performances given perfect classification.

Here, we measure the classification accuracies of the models in Table~\ref{tab:main} of the main paper, to complete the analysis. The performances are reported in Table~\ref{tab:main_cls}. There are in general great fluctuations in the classification results (26.8\% to 74.5\% on CUB). This is because we have selected the hyperparameters for each model that maximize the localization performances on \trainfullsup split. In many cases, the best localization performances are achieved at early epochs, before the classifiers are sufficiently trained (see also \S\ref{appendix:learning_curves} and Figure~\ref{fig:wsol_learning_curves}). The result signifies that localization and classification performances may not necessarily correlate and, therefore, localization-only metrics like \maxboxacc and \pxap must be used for model selection and evaluation of WSOL methods.

\input{tables/main_results_v2}

\subsection{Reproducing prior WSOL results}
\label{appendix:reproducing}

We also summarize reported results in prior WSOL papers~\cite{CAM,HaS,ACoL,SPG,ADL,CutMix} along with our reproduced results in Table~\ref{tab:previous_current_results}. While our main evaluation metrics are the classification-disentangled GT-known measures (\S\ref{subsec:evaluation_metrics} in main paper), we also report the \textit{top-1 localization} metrics that also measure the classification scores to match the reported numbers. Note that we use oracle $\tau$ for Top-1 localization accuracy. 

We experimentally observe that training epochs and batch sizes influence the localization accuracies ($\sim10$pp in \maxboxacc). However, the training details for each method are not given by the corresponding papers. All methods should share the same training budget for fair comparisons. Therefore, we fix our training epochs to ($10$, $50$, $10$) for (ImageNet, CUB, OpenImages) experiments, and fix the batch size to $32$ for all datasets. 

Following the prior methods~\cite{CAM, HaS, ACoL, SPG, ADL, CutMix}, we train all six methods by fine-tuning ImageNet pre-trained model. Specifically, we apply $10\times$ scale of learning rate to higher-level layers of backbone networks during training. We consider the last two layers for VGG, last three layers for InceptionV3, and last three residual blocks, and fully connected layers for ResNet as the higher-level layers.

Note that with GT-known metrics, our re-implementations produce better performances than the previously reported results (\eg $62.7\rightarrow 65.3$ for CAM on ImageNet with Inception backbone). This is perhaps because \maxboxacc and \pxap are based on the best operating thresholds.

Top-1 localization accuracies are reproduced well in general, except for the ADL: \eg $52.4\rightarrow 39.2$ for ADL on CUB with VGG backbone. This is due to the reduced training epochs compared to the original paper~\cite{ADL}, which results in a decreased classification accuracies.

\subsection{Score calibration and thresholding}
\label{appendix:score_calibration}

The operating threshold $\tau$ for the score map $s$ is an important parameter for WSOL. We show additional plots and visualizations to aid understanding. In Figure~\ref{fig:all_3_by_3_threshold_plots}, we show the \boxacc and \pxprec-\pxrec performances at different operating thresholds with diverse architectures and datasets. It extends the main paper Figure~\ref{fig:cam_threshold_and_pr_curves}. We observe again that the optimal operating thresholds $\tau^\star$ are vastly different across data and architectures for \boxacc. The \maxboxacc in each method are relatively stable across methods especially on ImageNet. OpenImages \pxprec-\pxrec curves do not exhibit big differences amongst WSOL methods, likewise.

In Figure \ref{fig:cam_value_dist}, we visualize score distributions for different WSOL methods. We observe that methods have different distributions of scores; ACoL in particular tends to generate flatter score maps. Comparing dataset, we observe that OpenImages tends to have more peaky score distributions. It is therefore important to find the optimal operating point for each method and dataset for fair comparison.

\begin{figure}
    \centering
    \includegraphics[width=\linewidth]{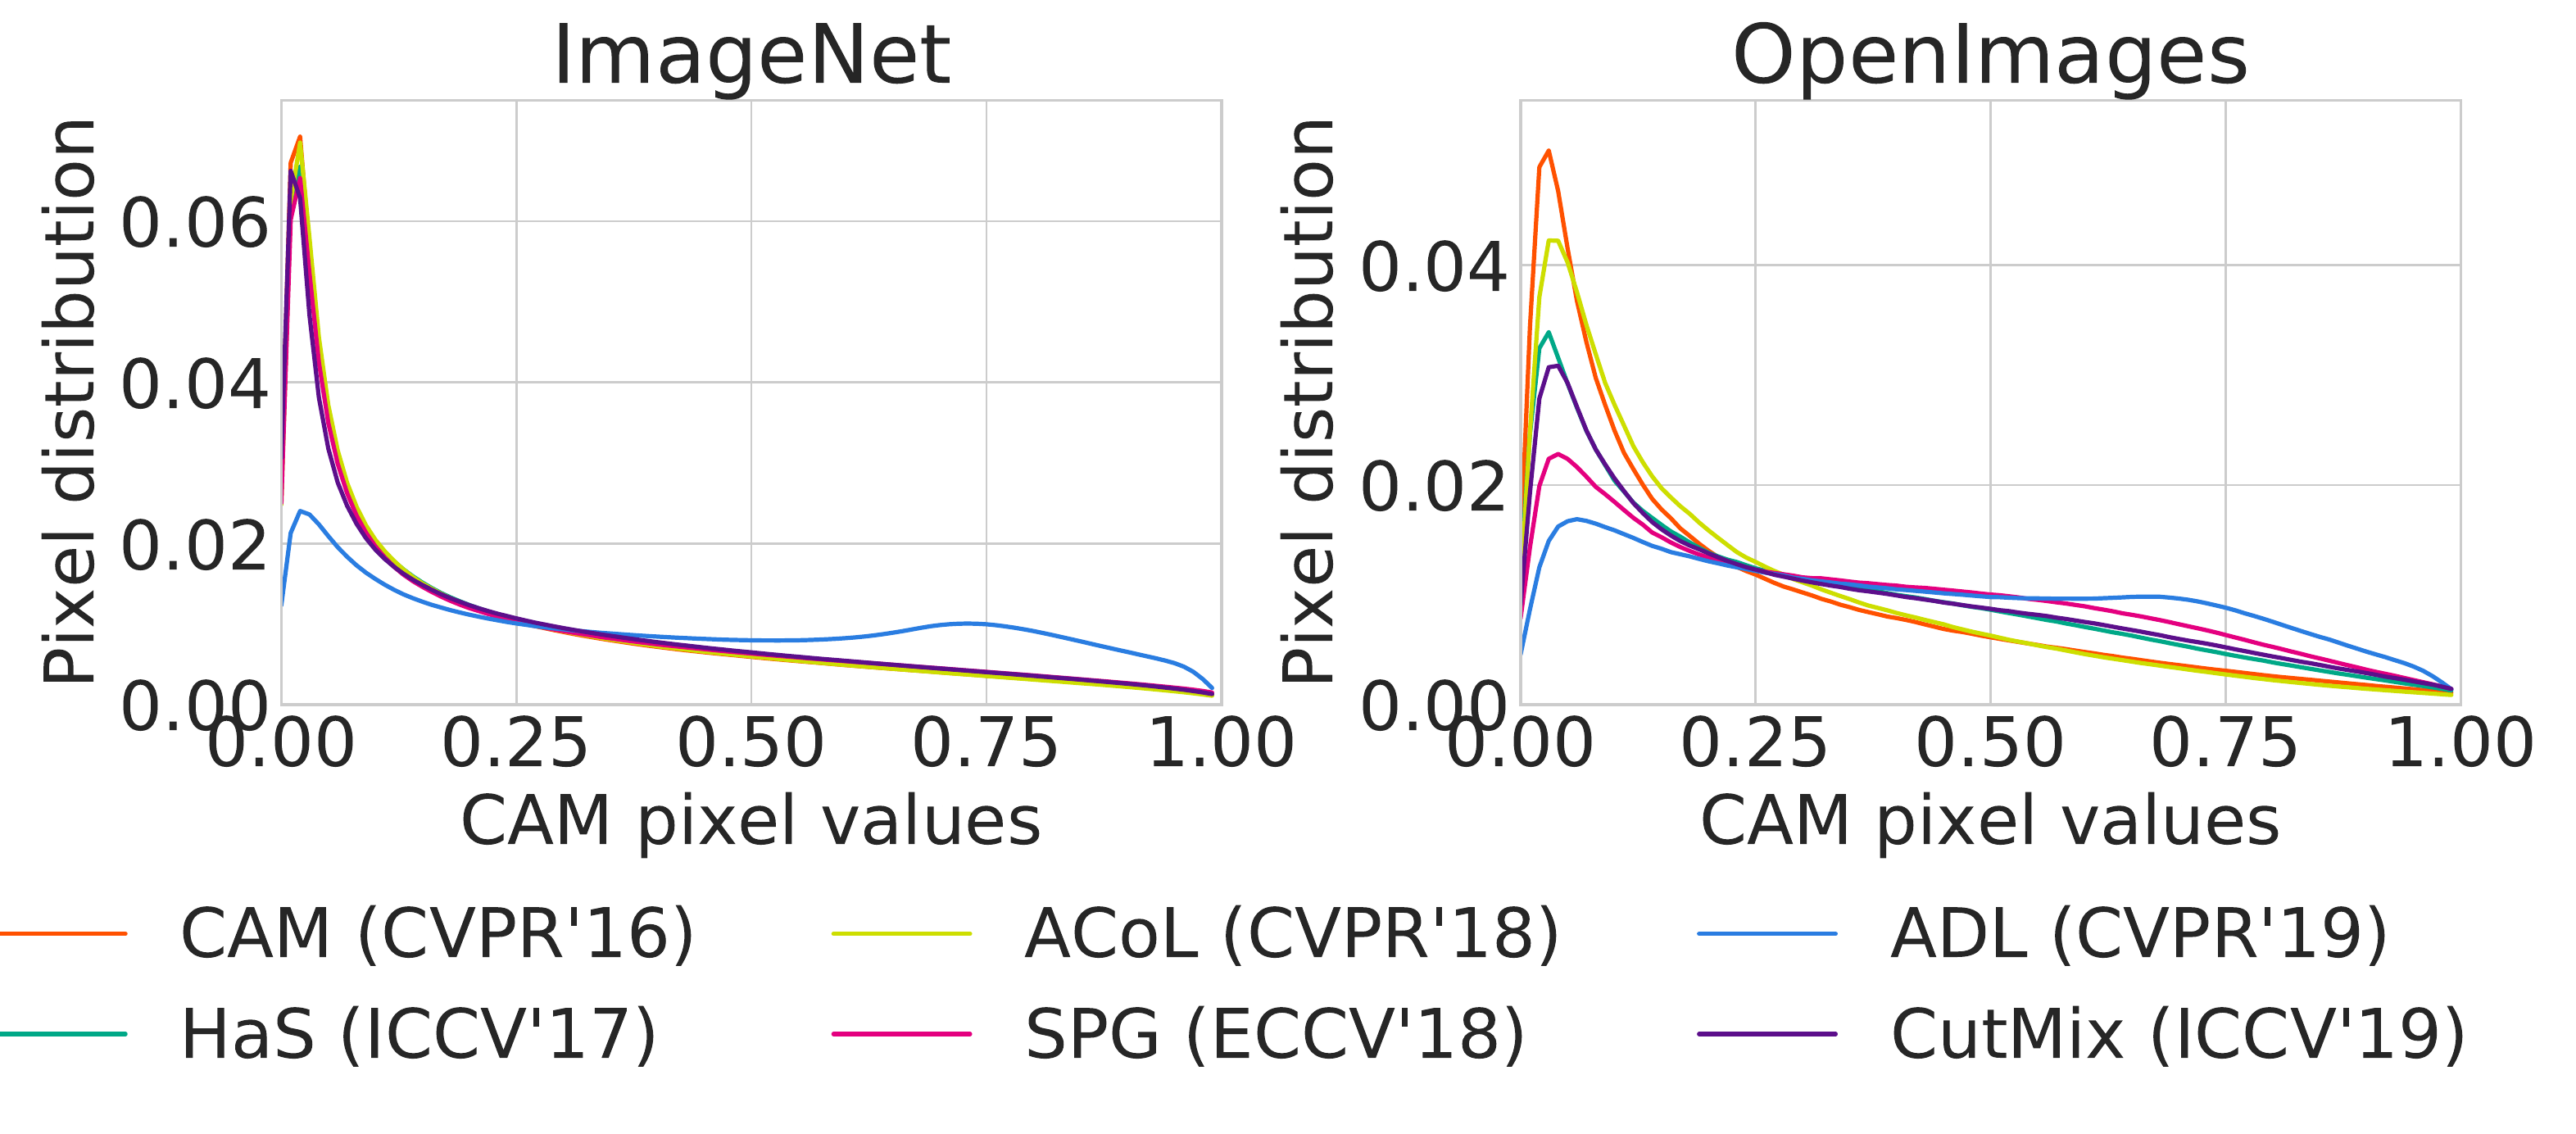}
    \caption{\small \textbf{CAM pixel value distributions.} On ImageNet and OpenImages \testfullsup.}
    \label{fig:cam_value_dist}
\end{figure}

We visualize more score maps in Figure~\ref{fig:score_map_visualization_imagenet},~\ref{fig:score_map_visualization_cub},~\ref{fig:score_map_visualization_openimages}; it extends the main paper Figure~\ref{fig:qualitative_cam_threshold}. We observe qualitatively different score maps in general across methods. However, the optimal IoU values are not as different and hard to predict just by visually looking at the samples. Again, it is important to have an objective way to set the thresholds $\tau$ in each case.

\subsection{Hyperparameter analysis}

We show the performance of all 30 hyperparameter search iterations on three datasets with three backbone architectures in Figure~\ref{fig:all_3_by_3_violin_plots}; it extends the main paper Figure~\ref{fig:wsol_robustness}. We observe similar trends as in the main paper. (1) Performances do vary according to the hyperparameter choice, so the hyperparameter optimization is necessary for the optimal performances. (2) CAM is among the more stable WSOL methods. (3) ACoL and ADL show greater sensitivity to hyperparameters in general. (4) CUB is a difficult benchmark where random choice of hyperparameters is highly likely to lead to performances worse than the center-Gaussian baseline.

\subsection{Learning Curves.}
\label{appendix:learning_curves}

We show the learning curves for CUB, ImageNet, OpenImages in Figure~\ref{fig:wsol_learning_curves}. We observe that the performances converge at epochs ($10$, $50$, $10$) for (ImageNet, CUB, OpenImages); the number of epochs for training models is thus sufficient for all methods. Note that learning rates are decayed by 10 every ($3$, $15$, $3$) epochs for (ImageNet, CUB, OpenImages). For the most cases, performance increases as the training progresses. However, in some cases (\eg CUB, SPG and OpenImages, CAM cases), best performances have already achieved at early iteration. That is, classification training rather hurts localization performance. Analyzing this is an interesting future study.  

\subsection{Evaluating WSOL methods with \newmaxboxacc}
\label{appendix:newmaxboxacc}

We re-evaluate six recently proposed WSOL methods with \newmaxboxacc, and the results are shown in Table~\ref{tab:main_v2}. All training configurations but evaluation metrics are the same as those of the main paper. We evaluate the last checkpoint of each training session. We obtain the same conclusions as with the original metric, \maxboxacc: (1) there has been no significant progress in WSOL performances beyond vanilla CAM~\cite{CAM} and (2) with the same amount of fully-supervised samples, FSL baselines provide better performances than the existing WSOL methods.

\clearpage
\input{tables/ranking_preservation_iid.tex}
\input{tables/all_3_by_3_threshold_plots.tex}
\input{tables/all_6_by_3_scoremaps.tex}
\input{tables/all_3_by_3_violin_plots.tex}
\input{tables/all_3_by_3_learning_curve.tex}
